# Supplementary material for: Sink-rise dynamics of horizontally oscillating active matter in granular media: Theory
Source: arXiv:2006.04160 source file (2020-06-07)
Supplement: Supplementary file 1 [file SuppMat.pdf]

# Sink-rise dynamics of horizontally oscillating active matter in granular media: Theory

## Supplementary information

Liu Ping,[1,2] Xianwen Ran,[1] and Raphael Blumenfeld[2,*]
[1] *National University of Defense Technology, Changsha 410073, China*
[2] *Cavendish Laboratory, JJ Thomson Avenue, Cambridge CB3 0HE, UK*

**The simulated system**
The numerical simulations were based on the open source software LIGGGHTS and the system setup is shown in Fig. 1 in the main text. For the inter-particle contact force, we used the Hertzian model:

$$\vec{F} = (k_n {\delta_n}^{3/2} - \gamma_n {\delta_n}^{1/4} v_n)\hat{n} + F_t \hat{t} \ , \tag{1}$$

where

$$F_t = \begin{cases} k_t {\delta_n}^{1/2} \delta_t - \gamma_t {\delta_n}^{1/4} v_t, & k_t |\delta_t| \le \mu |F_n| \\ -\mu F_n, & k_t |\delta_t| > \mu |F_n| \ . \end{cases} \tag{2}$$

Here, $\delta_i$ and $v_i$ are the components of the overlap displacement from the beginning of contact and the relative velocity of the particles in the $i$th direction, $\hat{n}$ is a unit vector in the normal direction to the contact plane and $\hat{t}$ is a unit vector in the contact plane along $\delta_t$. $\mu$ is the solid friction coefficient. For the contact interaction we assumed standard glass beads values: Young's modulus, $E = 5 \times 10^6$Pa, Possion's ratio $\nu = 0.3$, restitution coefficient $e = 0.8$, and friction coefficient $\mu = 0.5$. All the other parameters are listed in Table I.

**Determination of the vertical velocity**
To determine the momentary vertical velocity, we note that while AO overall has an upward trajectory, there is still an oscillation between rising and sinking with period $T/2$ underlying this upward movement. During the period where AO has an overall descending trajectory, the same movement pattern of underlying oscillations can be observed. We then choose the minimal depth of the AO at the first stroke, $z_0 \equiv z(t_0)$, with $0 < t_0 < T/2$ and measure the depths, $z_k$, for all possible $t_k = t_0 + kT/2$. The 'momentary' velocity at time $t_k$ is defined as

$$\overline{v}_k = \frac{z_{k+1} - z_{k-1}}{T} \ , \tag{3}$$

which is a smoothed representation of the otherwise oscillatory velocity variable. We used $k = 3, 5$ and $7$, where possible, and made sure that the average does not depend on $k$.

**The displacements in the $y$-direction**
As can be seen in Fig. 1, the displacements in the $y$ direction are much smaller than both those in the $z$-direction and the smallest oscillation amplitude, 0.05m. This justifies the quasi-two-dimensional modelling of the system and the dynamics of the AO.

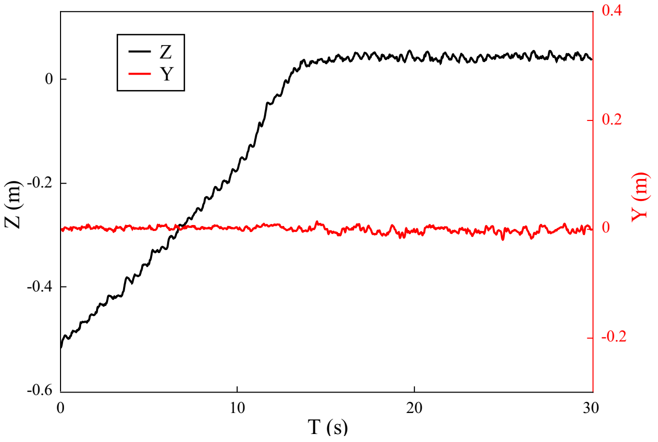


FIG. 1. Typical displacements of the AO in the $y$ and $z$ directions for amplitude $A = 0.1$m and frequency $f = 1$Hz. The former are very small compared to the latter and to the oscillation amplitudes.

**The maximum resistance force**
At low frequencies and all $A > 0.05$m, the AO experiences a linearly increasing resistance force with $x$ throughout a stroke up to a maximum that is proportional to the depth $h$ and independent of $A$ and $\omega$, as can be observed in Fig. 2. The observations are fitted well with $F_{R,max} = Ch$, with $C = 1770 \pm 10$N/m.

**Calculation of the resistance force on the AO**
We approximate the AO and the stagnant zone as a half-sphere and a cone, joined as sketched in Fig. 3. The local resistance force per unit area at depth $z$ is proportional to the hydrostatic-like pressure $K\rho_b g z$. Noting that $z = h - (L - x)\tan\alpha \sin\theta$, $r = (L - x)\tan\alpha$, and $dr = -\tan\alpha dx$, the force pushing against the infinitesimal area $rdrd\theta$ in Fig. 3 is

$$\begin{aligned} dF_R = {} & K\rho_b g \left[h - (L - x)\tan\alpha \sin\theta\right] \\ & \times (L - x)\tan\alpha \sin\alpha(-\tan\alpha)dx d\theta \ . \end{aligned} \tag{4}$$

Using $L = R/\tan\alpha$, we first integrate over $\theta$ on the shell

| Parameter | Particle-particle expression | Value | Particle-object expression | Value |
|---|---|---|---|---|
| $k_n$ | $\frac{E}{3(1-\nu^2)}\sqrt{d}$ | $26 \times 10^4 N \cdot m^{-\frac{3}{2}}$ | $\sqrt{\frac{4}{21}}\frac{E}{1-\nu^2}\sqrt{d}$ | $34 \times 10^4 Nm^{-\frac{3}{2}}$ |
| $k_t$ | $\frac{3(1-\nu)}{2-\nu}k_n$ | $32 \times 10^4 Nm^{-\frac{3}{2}}$ | $\frac{3(1-\nu)}{2-\nu}k_n$ | $42 \times 10^4 Nm^{-\frac{3}{2}}$ |
| $\gamma_n$ | $-\sqrt{\frac{5}{2}}\beta\sqrt{mk_n}$ | $0.18 kg \cdot s^{-1} \cdot m^{-\frac{1}{4}}$ | $-\sqrt{5}\beta\sqrt{mk_n}$ | $0.16 kg \cdot s^{-1} \cdot m^{-\frac{1}{4}}$ |
| $\gamma_t$ | $-\sqrt{\frac{5}{3}}\beta\sqrt{mk_t}$ | $0.11 kg \cdot s^{-1} \cdot m^{-\frac{1}{4}}$ | $-\sqrt{\frac{10}{3}}\beta\sqrt{mk_t}$ | $0.17 kg \cdot s^{-1} \cdot m^{-\frac{1}{4}}$ |

TABLE I. The parameters used in the simulation. Here, $d = R_i + R_j$ with $R_i$ and $R_j$ the radii of the particles in contact, $\beta = \ln e/\sqrt{\ln^2 e + \pi^2}$, and $m_i = 4\pi R_i^3 \rho_i/3$ is the mass of particle $i$, with $\rho_i$ its mass density.

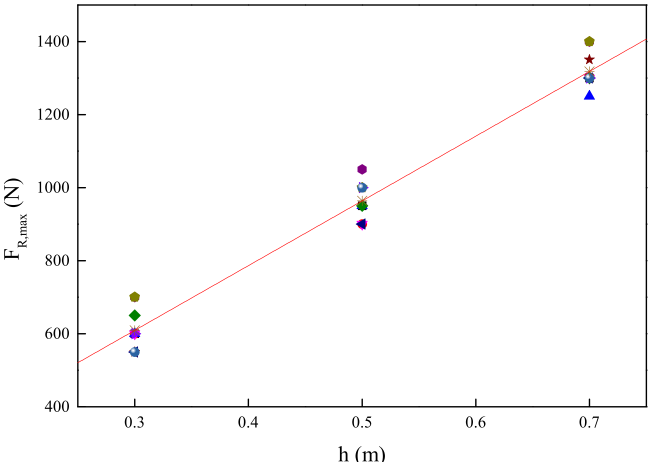


FIG. 2. The variation of the maximum resistance force, $F_{R,max}$ with depth. At each depth the data consist of all the cases satisfying $A\omega < v_c$: $(A, \omega) = (0.1, 1-5), (0.15, 1-3), (0.2, 1-2)$, and $(0.25, 1)$, many of which fall on top of one another at the resolution of our observations. The maximum fluctuates at every depth and is uncorrelated with either $A$ or $\omega$. A fit of the average of $F_{R,max}$ at each depth yields $F_{R,max} \approx Ch$, with $C = 1770 \pm 10$N/m.

at $r$ and then over $0 \leq x \leq R/\tan\alpha$, to obtain

$$F_R = -K\rho_b g R^2 h \sin\alpha \ , \tag{5}$$

with the sign indicating action against the direction of motion. Using the observed linear increase of $F_R$ with $x$ for $A\omega \leq v_c$ along the forward stroke, $F_R = Ch\left[A + x(t)\right]/(2A)$, we obtain the time-dependence of $\alpha$:

$$\sin\alpha = \frac{C\left(1 + \sin\omega t\right)}{2K\rho_b g R^2} \ . \tag{6}$$

**Calculation of the lift force on the AO**

The lift force is the sum total of the vertical component of the resistance as the inclined surface of the AO pushes against the medium. From Fig. 3, decomposing $dF_R$, the component normal to the surface is

$$dn = K\rho_b g z \frac{dx}{\cos\alpha} r d\theta \tag{7}$$

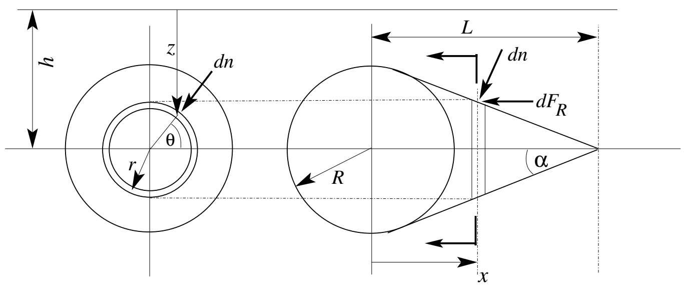


FIG. 3. The resistance force on the AO in the $x$-direction.

and the vertical component of this force is $dF_z = \sin\theta\cos\alpha\, dn$. Integrating over $x$ and $\theta$ between the same limits as above, we obtain

$$F_z = -\frac{\pi R^3}{3} K\rho_b g \sin\alpha\cos^2\alpha \ , \tag{8}$$

with the negative sign indicating action against the direction of gravity. The lift force is the result of the differential pressure across the cone's surface. Comparing to (5), we have

$$|F_z| = \frac{\sin 2\alpha}{6}\left(\frac{R}{h}\right)|F_R| \ . \tag{9}$$

**Effects of parameters**

We carried out simulations to study the effects of AO and media properties on the rising or sinking rate. We varied the AO-to-bed particle density ratio, AO-to-bed particle size ratio, and friction coefficient between bed particles and the AO. The effects of these on the rising or sinking rates are the following.

*AO-to-bed particle density ratio*

To test the effect of the AO-to-bed particle ratio of mass densities, we varied the AO's density from $\rho_m = 1000$Kg/m$^3$ to 7500Kg/m$^3$, for a fixed bed particle mass density of 2500Kg/m$^3$. As expected, we observed that the sinking rate increases and the rising rate decreases when the AO gets heavier. This effect is shown in Fig. 4 for amplitude 0.1m and frequency 15Hz.

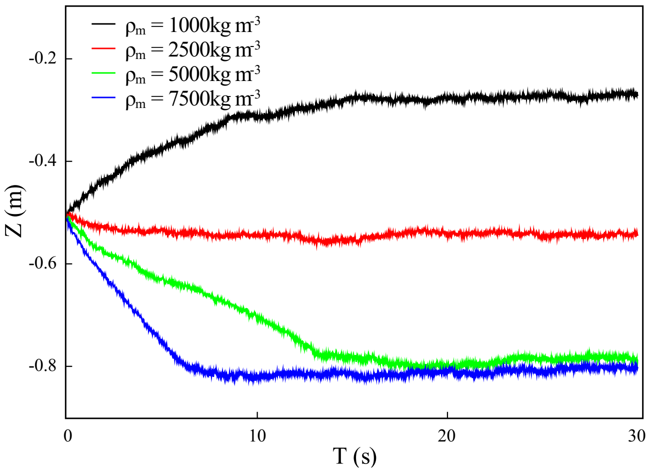


FIG. 4. The AO rises more slowly and sinks more quickly as its density increases.

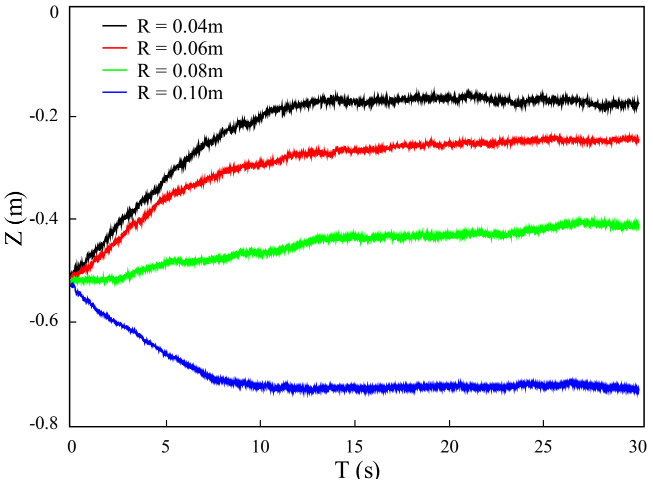


FIG. 5. The AO rises more slowly and sinks more quickly as its size increases.

*AO-to-bed particle size ratio*

To test the size ratio effect, we varied the AO-to-bed particle radius ratio from 4 to 10, for a fixed bed particles radius of 0.01m, $\rho_m = 5000\text{Kg/m}^3$ and $\rho_b = 2500 \times 0.69\text{Kg/m}^3$. We observe that the sinking rate increases and the rising rate decreases as the AO gets larger, as we exemplify in Fig. 5 for $A = 0.1$m and $f = 10$Hz.

*Friction coefficient*

To test the effect of intergranular friction on the rising and sinking dynamics, we varied the friction coefficient between the AO and bed particles from $\mu = 0.1$ to $\mu = 0.9$. We observed that the AO's rising rate increases with $\mu$ up to 0.5, at which value it saturates. This effect is exemplified for $A = 0.1$m and $f = 1$Hz in Fig. 6 - the rising rates at $\mu = 0.5, 0.7, 0.9$ are practically the same.

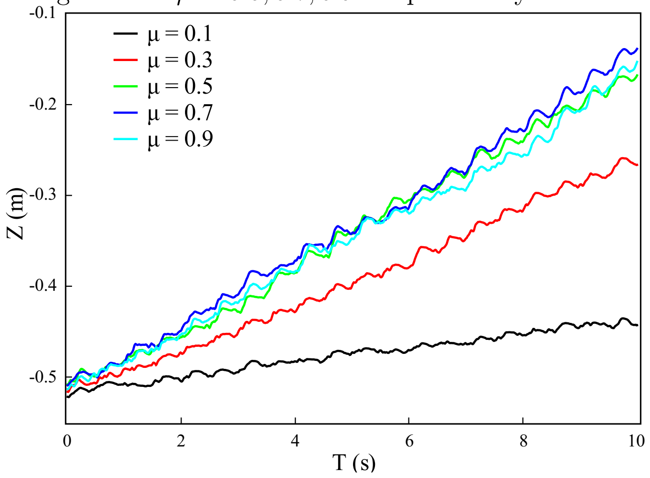


FIG. 6. The AO rises more quickly as the interparticle friction, $\mu$, increases from 0 up to 0.5. Increasing it further does not affect the rising.
